# Supplementary material for: InstaDrive: Instance-Aware Driving World Models for Realistic and Consistent Video Generation
Source: arXiv:2602.03242 source file (2026-02-03)
Supplement: Supplementary file 1 [file comparision-appendix.tex]

\begin{figure*}[t]
\centering
\begin{minipage}{0.50\linewidth}
    \centering
    \includegraphics[width=\linewidth]{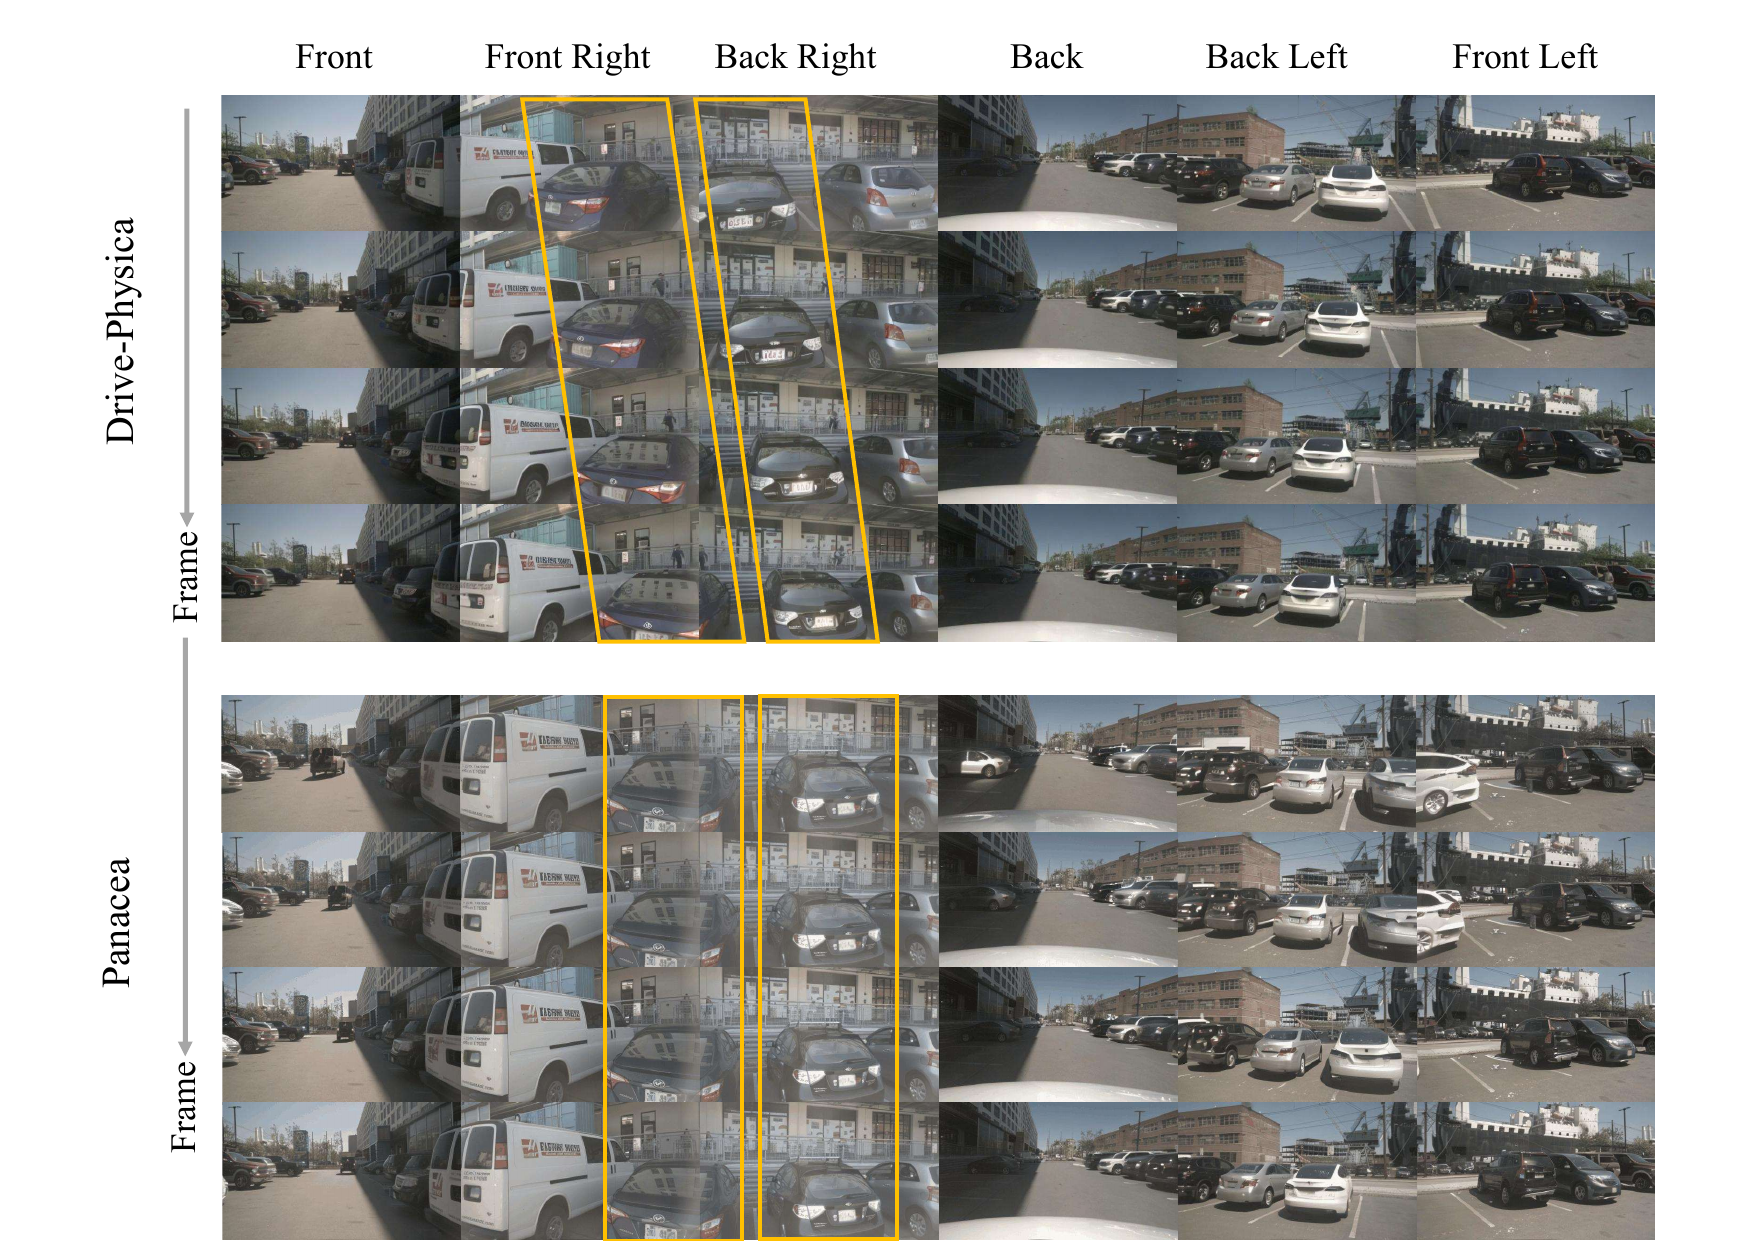} 
    \subcaption{Relative Motion Understanding.}
    %\label{fig:subfig3}
\end{minipage}\hfill
\begin{minipage}{0.50\linewidth}
    \centering
    \includegraphics[width=\linewidth]{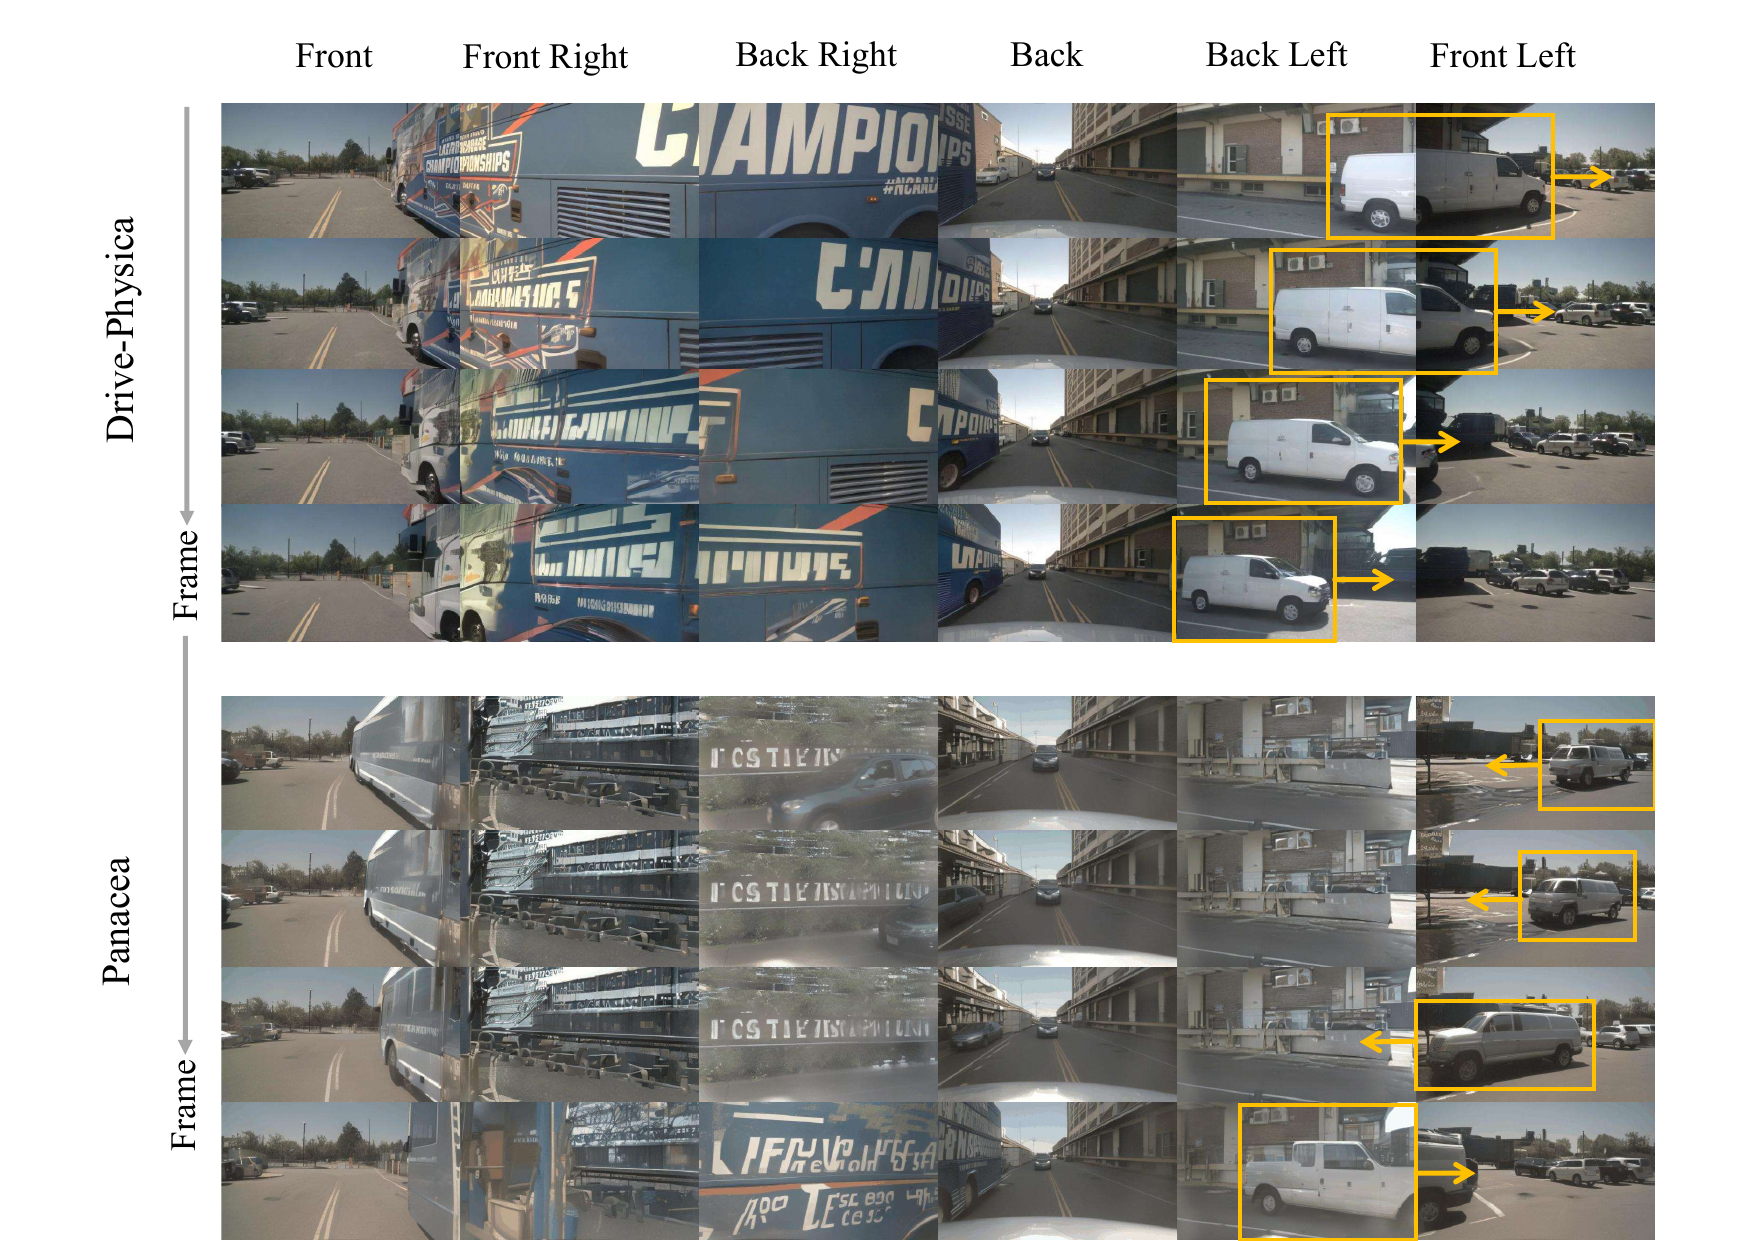} 
    \subcaption{Temporal Consistency.}
    %\label{fig:subfig1}
\end{minipage}\hfill
\begin{minipage}{0.49\linewidth}
    \centering
    \includegraphics[width=\linewidth]{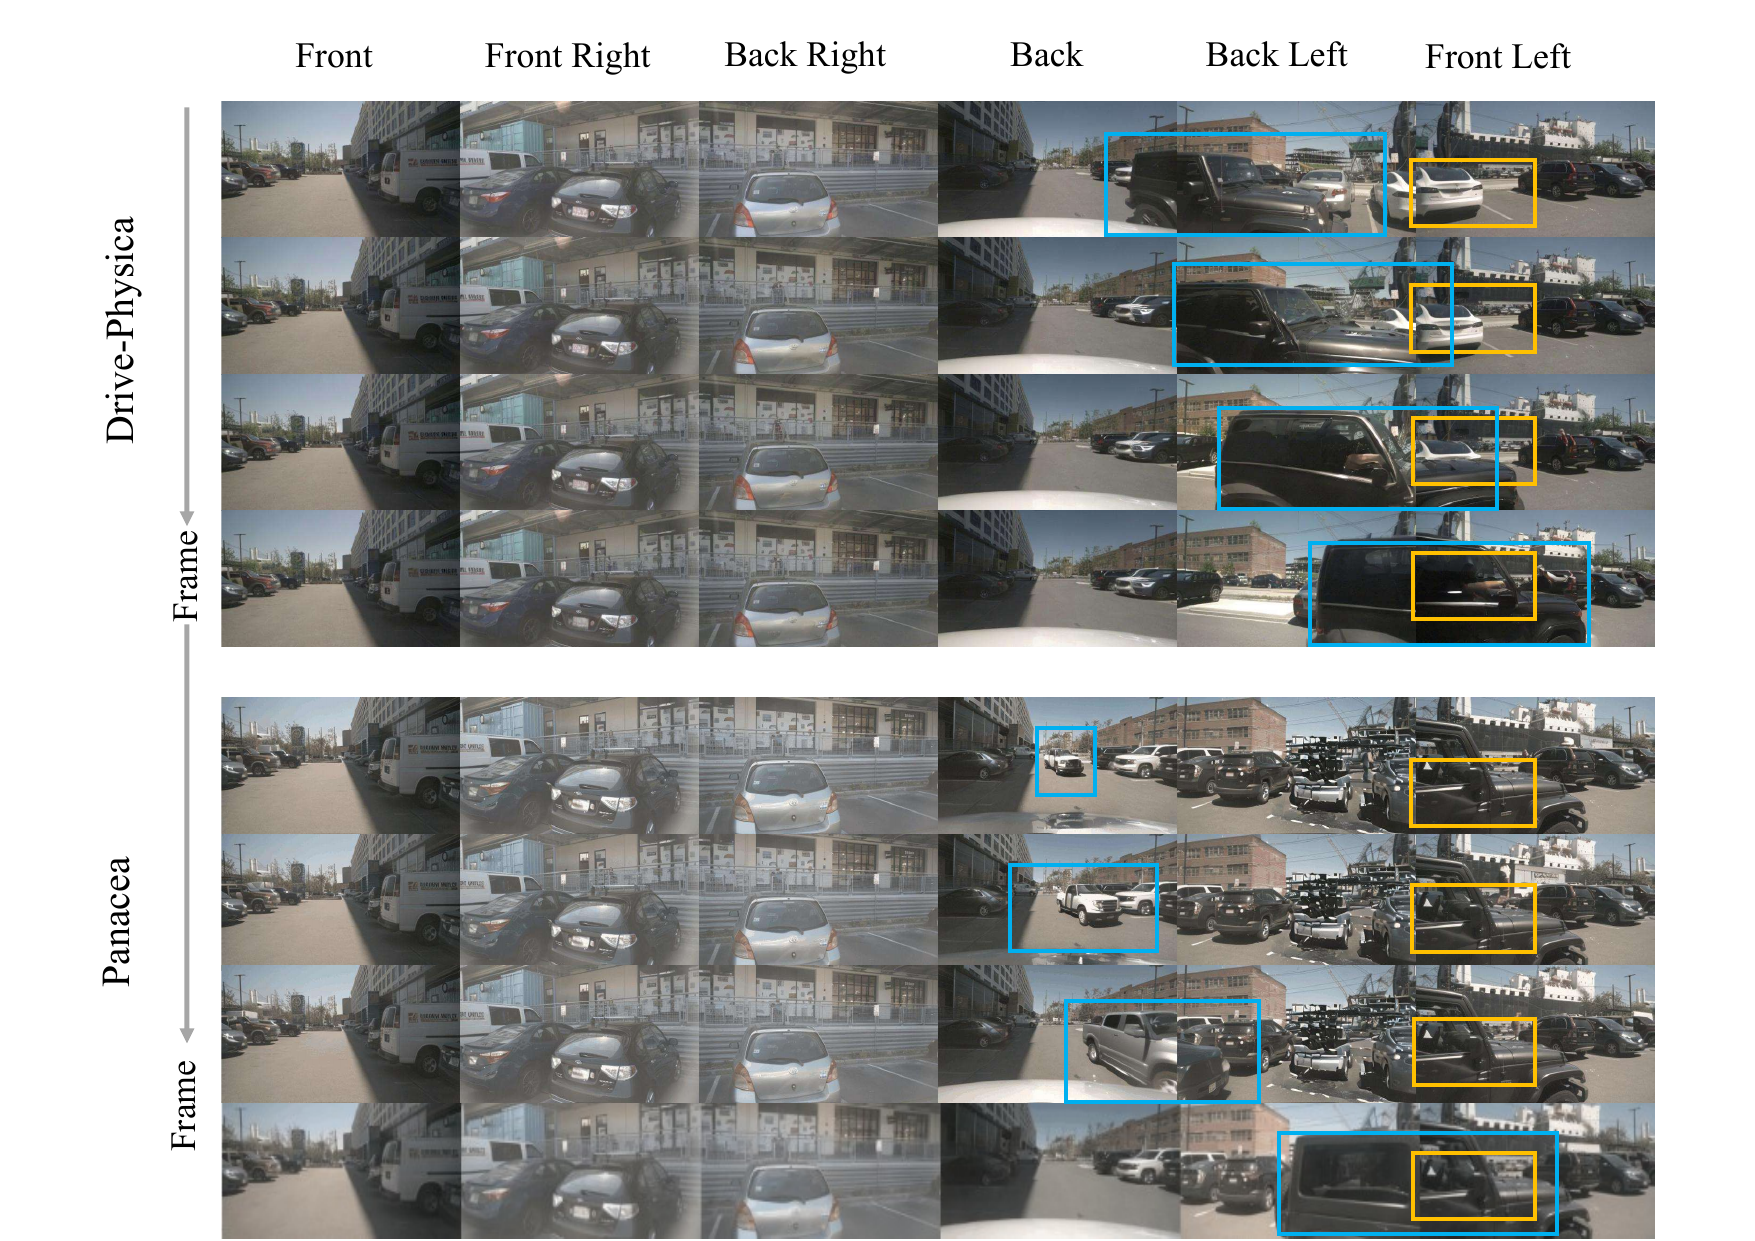} 
    \subcaption{Occlusion Hierarchy.}
    %\label{fig:subfig2}
\end{minipage}
\begin{minipage}{0.49\linewidth}
    \centering
    \includegraphics[width=\linewidth]{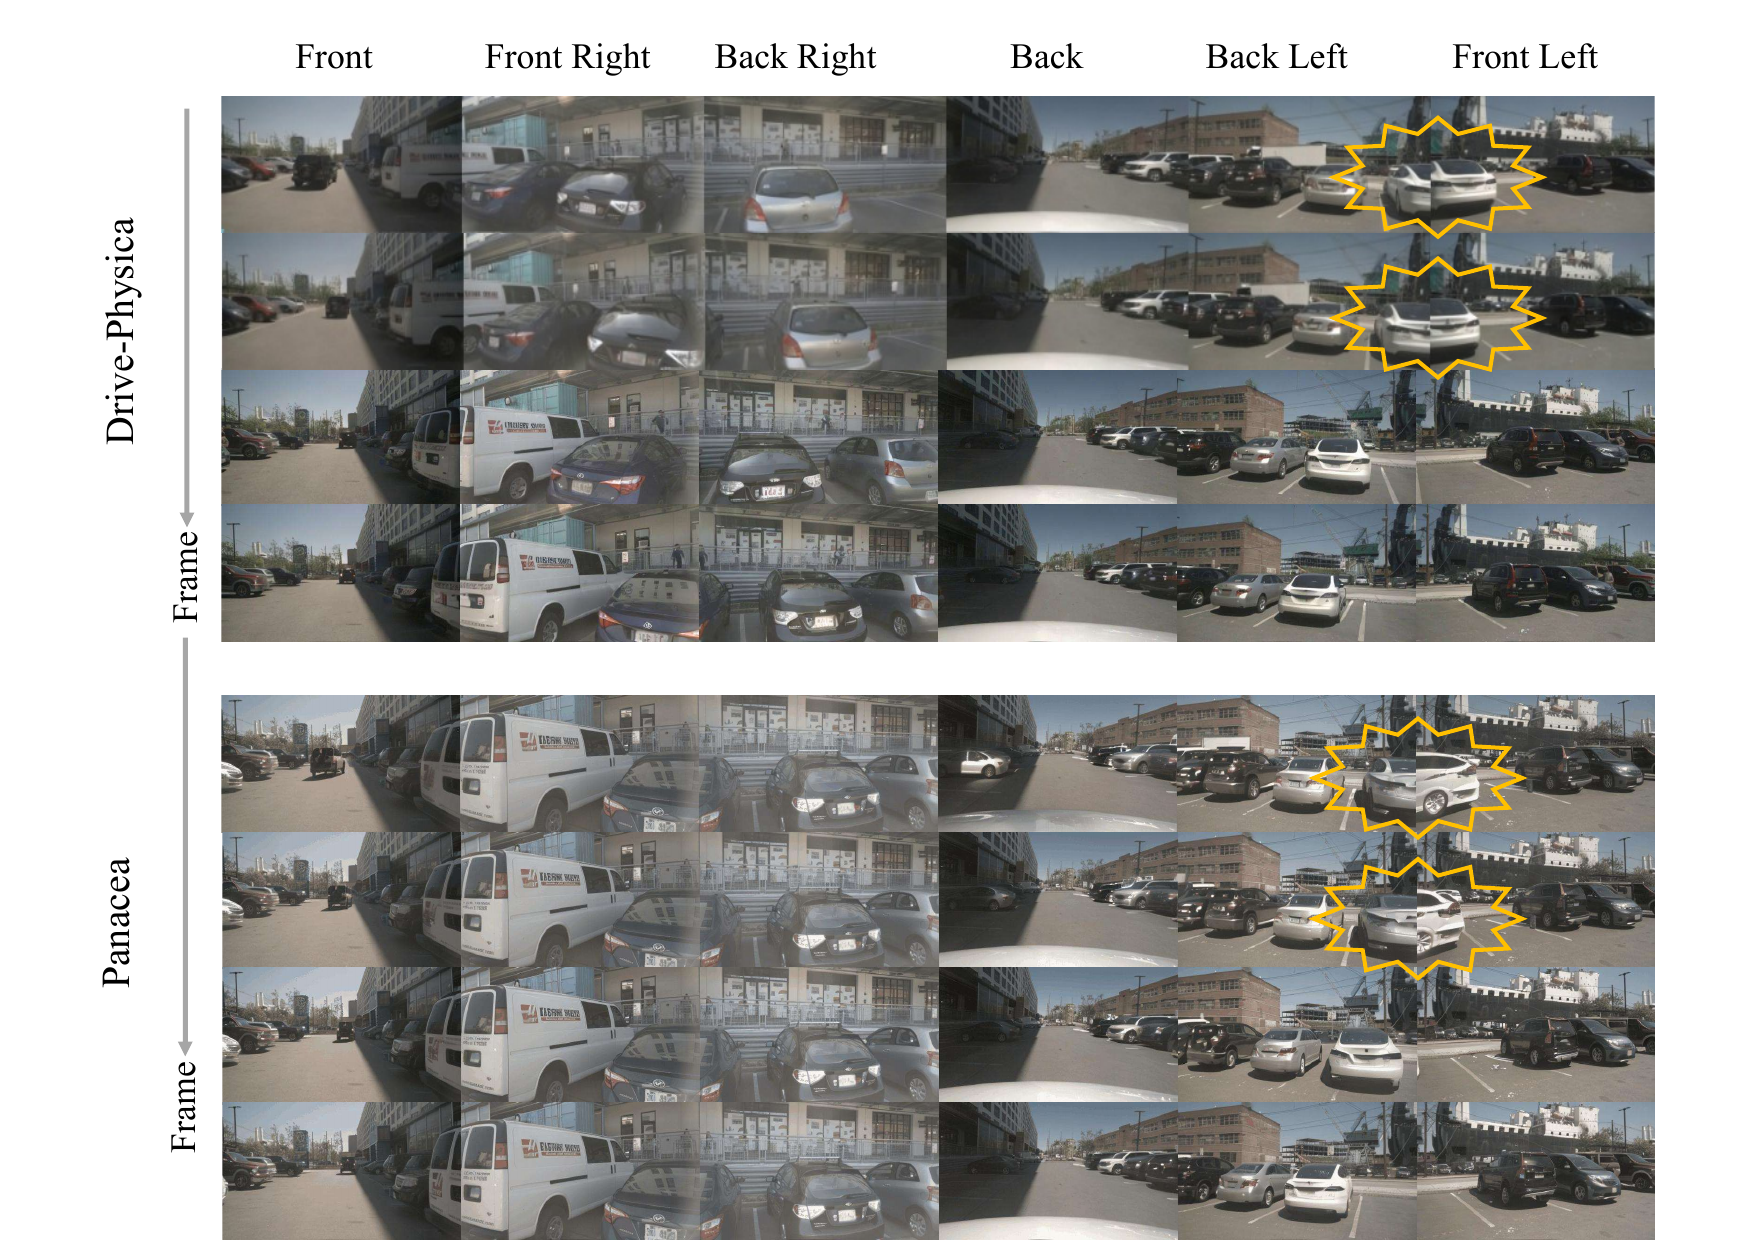} 
    \subcaption{Spatial Consistency.}
    %\label{fig:subfig4}
\end{minipage}
\caption{Qualitative comparison of videos generated by our model and Panacea, the current state-of-the-art method. 
\textbf{(a)} \textbf{Relative Motion Understanding:} As the ego vehicle moves forward, the background and foreground cars should appear to move backward relative to it.  
In Panacea, the black car fails to exhibit correct relative motion and does not move backward as expected relative to the ego vehicle.  
In contrast, our model accurately captures the relative motion of each instance, demonstrating a precise understanding of both the vehicle coordinate system and the world coordinate system.
\textbf{(b)} \textbf{Temporal Consistency:} In Panacea, the white car's shape and orientation (e.g., the direction of the car's front head) change over time. In contrast, our model preserves the white car's attributes throughout the frame, demonstrating superior temporal consistency.
\textbf{(c)} \textbf{Occlusion Hierarchy:} The stationary car (controlled by the orange box condition) is positioned farther from the ego vehicle, while the moving car (controlled by the blue box condition) is closer.  
In Panacea, the generated video incorrectly places the farther stationary car in front, obstructing the closer moving car, therefore violating the expected occlusion hierarchy.  
In contrast, our model correctly renders the closer moving car in front, with the farther stationary car appropriately occluded, demonstrating a superior understanding of occlusion hierarchy.
\textbf{(d)} \textbf{Spatial Consistency:} In Panacea, the white car exhibits different shapes in different views, reflecting spatial inconsistency. 
In contrast, our model maintains consistent spatial representation across views, ensuring coherence throughout the view. 
%Full-length videos are available on our project page in the supplementary materials \textcolor{red}{./drivephysica/page.html}.
}
\label{fig:contrast}
\end{figure*}
