# Supplementary material for: InstaDrive: Instance-Aware Driving World Models for Realistic and Consistent Video Generation
Source: arXiv:2602.03242 source file (2026-02-03)
Supplement: Supplementary file 2 [file X_suppl.tex]

\clearpage
\setcounter{page}{1}
\maketitlesupplementary

\appendix

\section{More Experimental Details}  
\label{app: exp}

We provide a project page for additional video results: \url{https://metadrivescape.github.io/papers_project/InstaDrive/page.html}.

%\textcolor{red}{Please unzip the entire supplementary materials archive before opening the webpage. Tested OK on macOS and Windows 10 systems.}

\subsection{Training Details}
Our method is implemented based on OpenSora \cite{opensora}. 
Initially, we train for 20k iterations on the front-view videos from the NuScenes training set. Next, to adapt to multi-view positional encoding, we froze the backbone and fine-tuned the patch embedder for 2k iterations. Finally, we added all the control modules and trained the entire model for 100k iterations with a mini-batch size of 1. All training inputs were set to 16x256x448 and performed on 8 A100 GPUs. Additionally, during training, we set a 0.2 probability of not adding noise to the first frame and assigned a timestep of 0 to the first frame, enabling the model to have image-to-video generation capability. As a result, during testing, the model can autoregressively iterate. Experimental results show that our method can stably generate over 200 frames.% and the project webpage included.

\subsection{Perception Evaluation Details}
In Tab.~\ref{tab:perception_augment}, StreamPETR was re-implemented from official config due to resolution differences with Panacea. Stronger baselines are harder to surpass, further highlighting our data’s effectiveness.

%\subsection{Framework Details}

% We did not use OpenSora V1.2, even though this version offers better performance. This is because the VAE in V1.2 also compresses the temporal dimension, and we found that this temporal compression leads to significant detail loss when generating driving scenes. The likely reason is that driving scenarios typically involve fast motion, and compressing the temporal dimension results in the loss of too much information. How to achieve reasonable spatiotemporal compression for generating autonomous driving scenes might also be a topic worth further research.

\section{More Quantitative Results}

\subsection{Evaluation on Planning Task.} 
% planning
\label{app:planning}
We also assess our model in the planning task in autonomous driving.
A high-quality planning system not only perceives the current environment but also maintains stable temporal understanding of dynamic objects (e.g., pedestrians, vehicles) to generate smooth and safe trajectories. 
Therefore, planning task performance serves as a comprehensive measure of both instance-level temporal consistency and spatial geometric fidelity. 

To validate our approach, we evaluate the generated nuScenes validation data using pretrained planning model UniAD \cite{shi2016uniad} in Tab.~\ref{tab:planning}.
The L2 loss and collision rates closely match the performance of the original data, demonstrating clear benefits from improved temporal consistency and spatial fidelity.

\begin{table}[tb]
    \centering
    \footnotesize
    \resizebox{0.475\textwidth}{!}{
        \setlength{\tabcolsep}{4pt}
        \begin{tabular}{c |c c c c |c c c c }
            \toprule
            \multirow{2}{*}{Eval Data} & \multicolumn{4}{c|}{L2(m)$\downarrow$} & \multicolumn{4}{c}{Col. Rate$\downarrow$} \\
            & 1s & 2s & 3s & Avg. & 1s & 2s & 3s & Avg. \\
            \hline
            Oracle & 0.48 & 0.96 & 1.65 & 1.03 & 0.0005 & 0.0017 & 0.0071 & 0.0031 \\
            \titleDef~ & 0.67 & 1.54 & 2.69 & 1.63 & 0.0033 & 0.0095 & 0.0189 & 0.0105 \\ 
            \bottomrule
        \end{tabular}
    }
    \caption{Comparison on planning task using the pre-trained planning model UniAD \cite{shi2016uniad}.
    We resize all generated images to 900×1600 to ensure a unified evaluation standard. The L2 loss and collision rates closely match the performance of the original data, highlighting the benefits of enhanced temporal consistency and spatial fidelity.
    }
    \label{tab:planning}
\end{table}

\subsection{Ablation Study for SGA}
%In Tab. \ref{tab:ablation_sga}, we isolate the impact of \textit{box projection} and \textit{depth injection} in the Spatial Geometric Aligner module.
We conduct ablation on the SGA module by gradually removing its two components: depth injection and box projection.
As shown in Tab.~\ref{tab: ablation}, removing both causes a large drop of 3.20 in NDS and a big increase of 187 in IDS, confirming the importance of SGA module.
Individually, removing box projection leads to a larger NDS drop, while removing depth injection results in more ID switches, indicating their respective contributions to spatial localization and temporal consistency.

% \vspace{-0.8em}
% \begin{table}[htbp]
%     \centering
%     \footnotesize
%         \centering
%         \resizebox{0.48\textwidth}{!}{
%         \setlength{\tabcolsep}{4pt}
%         \begin{tabular}{lcccc}
%             \toprule
%             Settings        & FVD$\downarrow$ & FID$\downarrow$ & NDS$\uparrow$ & IDS$\downarrow$ \\
%             \hline 
%             w/o SGA(Box) & 39.27 \textcolor{blue}{(+1.21)}& 4.07 \textcolor{blue}{(+0.11)} & 38.22 \textcolor{blue}{(-2.29)} & 628 \textcolor{blue}{(+92)}\\ 
%             w/o SGA(Depth)   & 40.46 \textcolor{blue}{(+2.40)} & 4.15 \textcolor{blue}{(+0.19)} & 39.13 \textcolor{blue}{(-1.38)} & 669 \textcolor{blue}{(+133)}\\
%             \bottomrule
%         \end{tabular}
%         }
%         \captionsetup{skip=2pt}
%         \caption{SGA ablation: isolate \textit{box projection} / \textit{depth injection}.}
%         \label{tab:ablation_sga}
%         \vspace{-1.5em}
% \end{table}

\subsection{Ablation Study in T2V Scenario}
\label{app: t2v}
We also conduct an ablation study in the T2V scenario to evaluate the effectiveness of two key modules—the Instance Flow Guider (IFG) module and the Spatial Geometric Aligner (SGA) module. The results are presented in Tab.\ref{tab: ablation2}.

\noindent \textbf{Instance Flow Guider.}
To assess the impact of the IFG module, we eliminate the instance flow injection. In the T2V mode, where no guidance is provided from the first frame, the IFG module plays a more critical role compared to its role in the (T+I)2V mode. As shown in Tab.\ref{tab: ablation2}, removing the instance flow injection leads to a significant degradation, with the FVD score increasing by $46.81$. This highlights the module’s importance in ensuring smooth and coherent video generation.

\noindent \textbf{Spatial Geometric Aligner.}
To evaluate the influence of the SGA module, we remove the injection of depth order and replace the box projection with box coordinates as the control signal. 
This ablation significantly impacts the model’s ability to accurately localize objects and understand spatial relationships. As demonstrated in Tab.\ref{tab: ablation2}, the absence of the SGA module results in a notable performance drop, further emphasizing its essential role in achieving high spatial fidelity.

\begin{table}[tb]
    \centering
    \footnotesize
        \centering
        \resizebox{0.475\textwidth}{!}{
        \setlength{\tabcolsep}{23pt}
        \begin{tabular}{lcc}
            \toprule
            Settings        & FVD$\downarrow$ & FID$\downarrow$  \\
            \hline
            \rowcolor[gray]{.9} 
            \titleDef~   & 107.50 & 12.91 \\
            \hline
            w/o Instance Flow Guider  & 154.31 \textcolor{blue}{(+46.81)} &  16.73 \textcolor{blue}{(+3.82)}\\ 
            w/o Spatial Geometric Aligner & 117.25 \textcolor{blue}{(+9.75)}& 14.52 \textcolor{blue}{(+1.61)}\\           
            \bottomrule
        \end{tabular}
        }
        \caption{Ablation study results in T2V scenarios on the generated nuScenes validation set.}
        \label{tab: ablation2}
\end{table}

\begin{figure*}[t]
\centering
% \begin{minipage}{\linewidth}
%     \centering
%     \includegraphics[width=\linewidth]{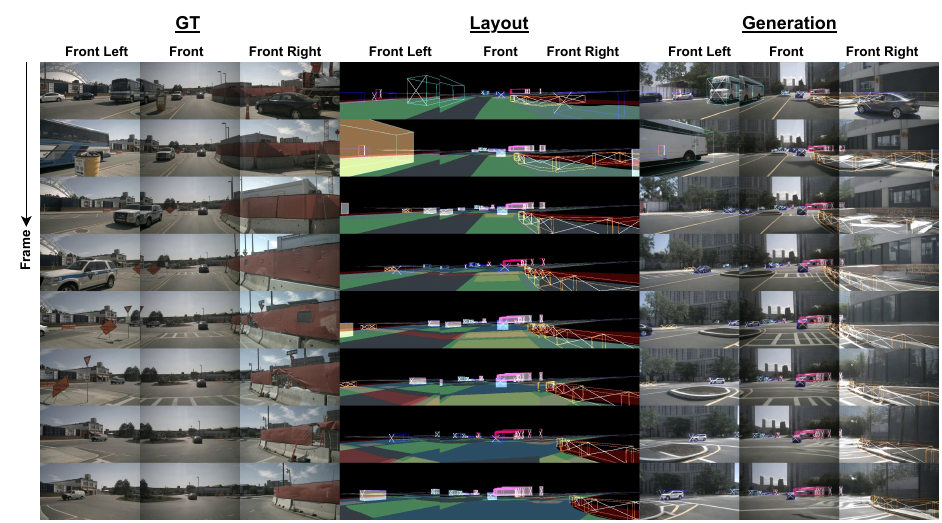} 
%     \subcaption{Relative Motion Understanding.}
%     \label{fig:subfig3}
% \end{minipage}\hfill
\begin{minipage}{\linewidth}
    \centering
    \includegraphics[width=\linewidth]{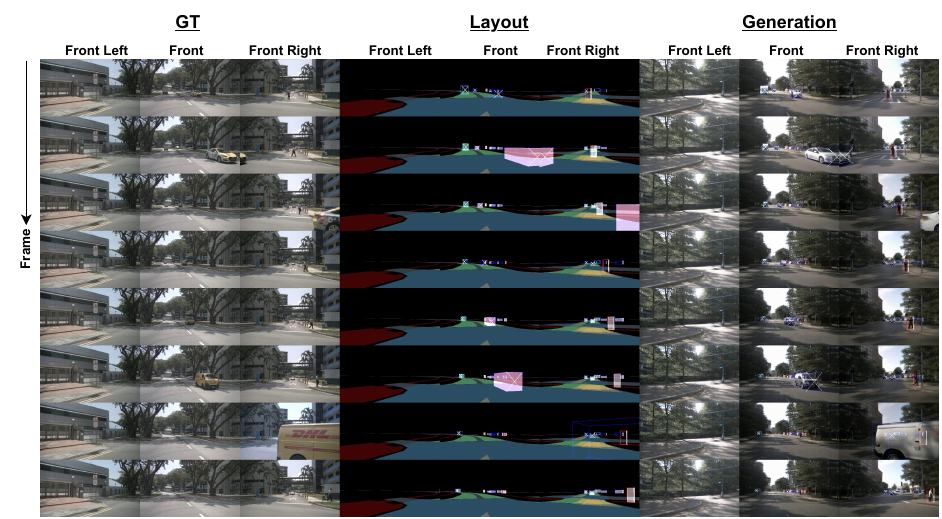} 
    \subcaption{Objects track their attributes maintaining temporal consistency.}
    \label{fig:subfig1_control}
\end{minipage}
\begin{minipage}{\linewidth}
    \centering
    \includegraphics[width=\linewidth]{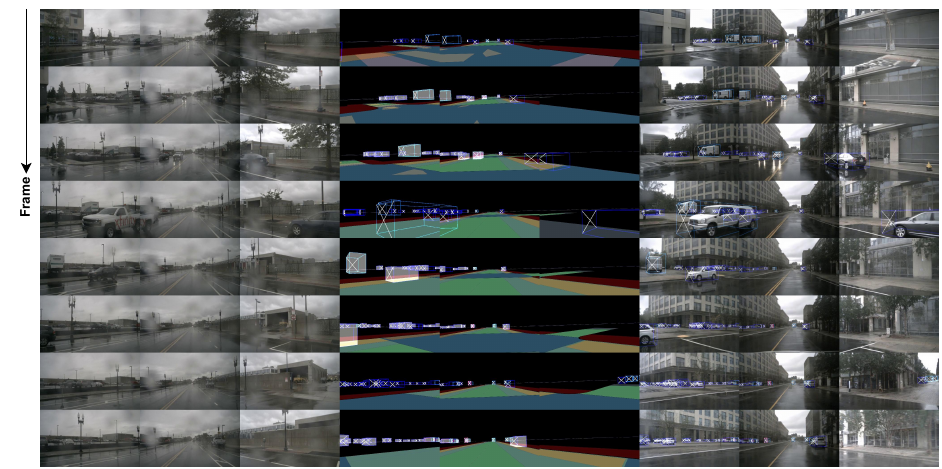} 
    \subcaption{Small and densely packed objects rendered at correct locations.}
    \label{fig:subfig2_control}
\end{minipage}
\caption{ Precise control mechanisms. We overlay the 3D bounding box projections onto the generated videos. The precision of control is reflected in: 
\textbf{(1)} Objects in the scene are accurately placed and sized to align with their \textit{projected bounding boxes}, as shown in \ref{fig:subfig1_control} and \ref{fig:subfig2_control}. 
\textbf{(2)} Drivable areas, sidewalks, and zebra crossings are faithfully generated following the \textit{road map projections}, as shown in \ref{fig:subfig1_control} and \ref{fig:subfig2_control}. 
\textbf{(3)} Objects track their previous attributes as guided by the \textit{instance flow}, ensuring temporal consistency across frames. As shown in Figure~\ref{fig:subfig1_control}, the pink-rendered instance flow directs the model to generate the white sedan, maintaining its consistent attributes over time.
\textbf{(4)} Small and densely packed objects are precisely rendered at their correct locations, following \textit{3D bounding box coordinates}, as shown in \ref{fig:subfig2_control}.
%Full-length videos are available on our project page in the supplementary materials \textcolor{red}{./drivephysica/page.html}
}
\label{fig:control}
\end{figure*}

\begin{figure*}[t]
\centering
\includegraphics[width=\linewidth]{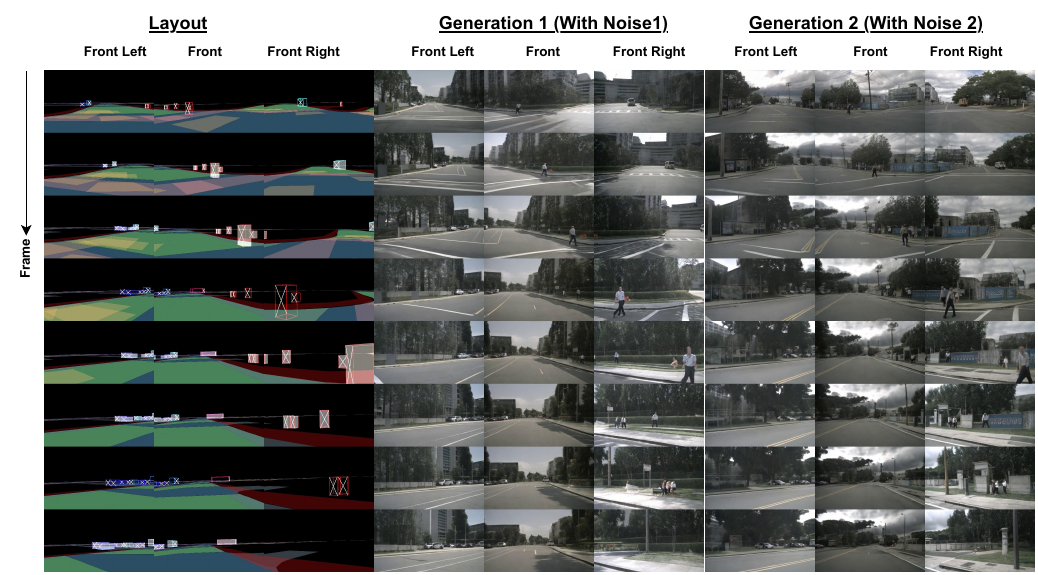} 
\caption{Diverse videos using \textbf{varying noise inputs} and \textbf{the same control conditions}. 
By introducing stochastic noise while maintaining consistent control signals—such as 3D bounding box coordinates, lane line projections, and instance flow—our model can produce a variety of videos that adhere to the defined constraints.
%Full-length videos are available on our project page in the supplementary materials \textcolor{red}{./drivephysica/page.html}
}
\label{fig:noise}
\end{figure*}

\section{More Visualization Results}
Here, we provide additional visualization results to showcase our model's strong ability to generate high-fidelity, realistic, and diverse multi-view driving videos. 
We sample 8 frames from each generated video as a demo to save space in the paper. Our model is capable of generating high-quality, long-duration driving videos through iterative processing. 
We provide a web page in the supplementary materials for additional results. Please refer to the webpage in the supplementary materials for visualization results.

\subsection{Prompt Edit}
\label{app:edit}
\titleDef~ enables video editing by modifying only the text prompt condition while keeping all other conditions fixed.  
In Fig.4 in main text, we demonstrate the model's editing capability by altering the weather and time of day in the text prompt. Specifically, we add "Sunny," "Rainy," and "Night" to the original text prompt, while maintaining other conditions such as camera pose, 3D bounding box coordinates, 3D bounding box projections, road map projections, and instance flow unchanged. The generated videos showcase high quality and effective editing:  
\begin{itemize}
    \item \textbf{Sunny}: Displays clear skies with sunlight shining on the scene, reflecting bright and vivid environmental details.  
    \item \textbf{Rainy}: Captures wet road surfaces and blurred camera views caused by raindrops, adding realistic weather dynamics.  
    \item \textbf{Night}: Depicts dimly lit scenes with streetlights and reduced visibility, accurately simulating nighttime driving conditions.  
\end{itemize}
These results emphasize the strong editing capability of \titleDef~, producing diverse and realistic driving videos with minimal changes to the input conditions.

\subsection{Control Precision}
\label{app:control}
\titleDef~ excels at generating videos that adhere closely to various control conditions, including 3D bounding box projections, road map projections, depth order, and instance flow.  
In Fig.~\ref{fig:control}, we overlay the 3D bounding box projections onto the generated videos to illustrate the precision of our control mechanisms.  The precision of control is reflected in:  
\begin{itemize}
    \item \textbf{Object alignment with bounding box projections}: Objects in the scene are accurately placed and sized to align with their projected bounding boxes, as shown in  Fig.~\ref{fig:control} (a)(b).  
    \item \textbf{Road and pedestrian area fidelity}: Drivable areas, sidewalks, and zebra crossings are faithfully generated following the road map projections, as shown in  Fig.~\ref{fig:control} (a)(b).  
    \item \textbf{Precision in dense and small objects}: Small and densely packed objects are precisely rendered at their correct locations, as shown in  Fig.~\ref{fig:control} (b).  
    \item \textbf{Temporal consistency through instance flow}: Objects track their previous attributes as dictated by the \textit{instance flow}, enabling consistent temporal consistency across frames, as shown in  Fig.~\ref{fig:control} (a).  
\end{itemize}
These results highlight the superior control and fidelity of \titleDef~ in generating realistic and controllable driving videos.

\subsection{Carla-Generated Layout Control}  
\label{app:carla}
\titleDef~ demonstrates the ability to generate high-quality driving videos based on layout conditions provided by the Carla simulator \cite{Dosovitskiy17}, which include 3D bounding box projections, lane line projections, and scene description text prompts. 
The use of Carla-generated layouts addresses a critical limitation in real-world driving video datasets: the lack of diversity in scene types, especially for rare but critical events like lane cutting and sudden braking. 
By leveraging Carla's highly configurable simulation environment, we can create synthetic layouts that represent complex and diverse driving scenarios, such as multi-vehicle intersections, narrow streets, or sudden obstacles, which are difficult to capture in real-world data.  

In Fig.5 in main text, we showcase our model's ability to generate rare videos corresponding to these layouts.   
The generated videos highlight \titleDef's capacity to faithfully adhere to the control signals while producing realistic outputs. 
Moreover, by effectively handling corner cases, our approach bridges the gap in scene diversity, making it a valuable tool for training and validating driving models under challenging scenarios. 
The results demonstrate that \titleDef~ can not only replicate realistic conditions but also adapt seamlessly to a wide range of complex layouts generated by Carla, further enhancing its applicability in autonomous driving research.

\subsection{Diversity with Varying Noise}
\label{app:noise}

\titleDef~ demonstrates the ability to generate diverse driving videos from identical control conditions with varying noise inputs, as illustrated in Fig.~\ref{fig:noise}. By introducing stochastic noise while maintaining consistent control signals—such as 3D bounding box coordinates, lane line projections, and instance flow—our model produces a variety of plausible video outputs that adhere to the defined constraints.

\begin{figure*}[t]
\centering
\includegraphics[width=0.8\linewidth]{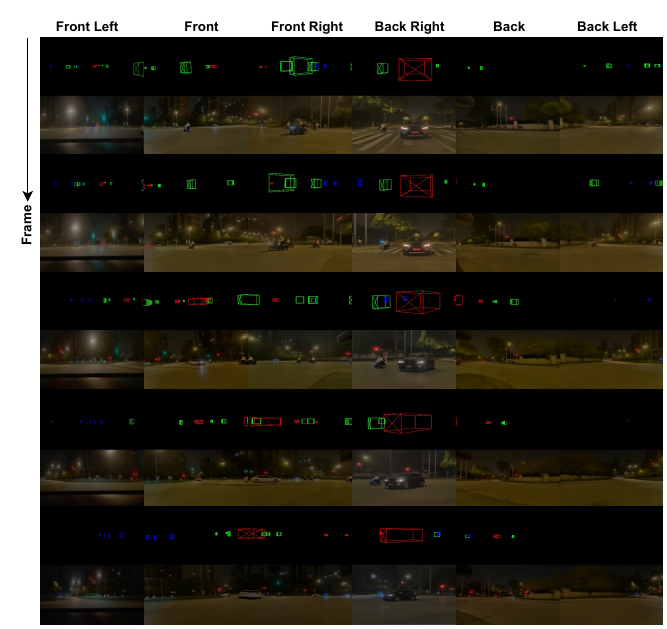} 
\caption{Results on private dataset.}
\label{fig:private}
\end{figure*}

\subsection{Results on our private dataset}
\label{app:private data}
In addition to public datasets, we trained on a 200 hour private dataset. The results, as shown in the Fig. \ref{fig:private}, demonstrate that we achieved similar generation quality and control performance as on nuScenes, highlighting the generalization capability of our method.

\section{Limitations}

Our work establishes a robust, physically informed framework for generating high-quality, multi-view driving videos, achieving state-of-the-art performance in both video generation quality and downstream perception task validation. However, certain limitations remain, mainly due to time and resource constraints.  

Currently, our model's design has not been exhaustively optimized, leaving room for improvement in the quality of the generated videos. For example, the training process is conducted at a relatively low spatial resolution of $256 \times 448$, which constrains visual fidelity. Scaling to higher resolutions would require fine-tuning the position embeddings to ensure compatibility, an aspect not yet addressed in this work.  

Future research could explore the integration of more advanced generative models, such as SD-XL ~\cite{DBLP:journals/corr/abs-2307-01952}, and develop more efficient methods to produce high-fidelity videos at larger spatial resolutions. Additionally, the computational cost of inference for InstaDrive is relatively high, which presents another avenue for improvement. Enhancing the efficiency of InstaDrive will be a key focus in future developments to make the model more practical for real-world applications.

\section{Backbone}
\label{section:preliminary}

% \textbf{Latent Video Diffusion Model~(LVDM).}
% The LVDM enhances the stable diffusion model ~\cite{ramesh2022hierarchical} by integrating a 3D U-Net, thereby empowering efficient video data processing. This 3D U-Net design augments each spatial convolution with an additional temporal convolution and follows each spatial attention block with a corresponding temporal attention block. It is optimized by employing a noise-prediction objective function:
% \begin{equation}
%     l_\epsilon = ||\epsilon - \epsilon_\theta(z_t, t, c)||^2_2,
%     \label{eq:training_objective}
% \end{equation}
% Here, $\epsilon_\theta(\cdot)$ signifies the 3D U-Net's noise prediction function. The condition 
% $c$ is guided into the U-Net using cross-attention for adjustment. Meanwhile, $z_t$ denotes the noisy hidden state, evolving like a Markov chain that progressively adds Gaussian noise to the initial latent state $z_0$:
% \begin{equation}
%     z_t=\sqrt{\bar{\alpha}_t}z_0 + \sqrt{1 - \bar{\alpha}_t}\epsilon, \quad\epsilon \sim \mathcal{N}(0, I),
%     \label{eq:add_noise}
% \end{equation}
% where $\bar{\alpha}_t = \prod_{i=1}^t(1-\beta_t)$ and $\beta_t$ is a coefficient that controls the noise strength in step $t$.

\noindent \textbf{Spatial-Temporal DiT (ST-DiT).}
We use Spatial-Temporal DiT (ST-DiT) \cite{peebles2023scalable} as our backbone, which introduces a novel architecture that merges the strengths of diffusion models with transformer architectures \cite{vaswani2017attention}. This integration aims to address the limitations of traditional U-Net-based latent diffusion models (LDMs), improving their performance, versatility, and scalability. While keeping the overall framework consistent with existing LDMs, the key shift lies in replacing the U-Net with a transformer architecture for learning the denoising function $\epsilon_\theta(\cdot)$, thereby marking a pivotal advance in the realm of generative modelling.

The ST-DiT architecture incorporates two distinct block types: the Spatial DiT Block (S-DiT-B) and the Temporal DiT Block (T-DiT-B), arranged in an alternating sequence. 
The S-DiT-B comprises two attention layers, each performing Spatial Self-Attention (SSA) and Cross-Attention sequentially, succeeded by a point-wise feed-forward layer that serves to connect adjacent T-DiT-B block. 
Notably, the T-DiT-B modifies this schema solely by substituting SSA with Temporal Self-Attention (TSA), preserving architectural coherence. 
Within each block, the input, upon undergoing normalization, is concatenated back to the block's output via skip-connections. Leveraging the ability to process variable-length sequences, the denoising ST-DiT can handle videos of variable durations.

During processing, a video autoencoder \cite{yu2023magvit} is first employed to diminish both spatial and temporal dimensions of videos. To elaborate, it encodes the input video $X \in \mathbb{R}^{T \times H \times W \times 3}$ into video latent $z_{0} \in \mathbb{R}^{t \times h \times w \times 4}$, where $L$ denotes the video length and $t = T, h = H / 8, w = W / 8$.  $z_{0}$ is next ``patchified", resulting in a sequence of input tokens $I \in \mathbb{R}^{t \times s \times d} $. Here, $s = hw/p^2$ and $p$ denote the patch size. 
$I$ is then forwarded to the ST-DiT, which models these compressed representations. 
In both SSA and TSA, standard Attention is performed using Query (Q), Key (K), and Value (V) matrices:
\[
Q = W_{Q} \cdot I_{norm}; K = W_{K} \cdot I_{norm}; V = W_{V} \cdot I_{norm},
\]

$I_{norm}$ is the normalized $I$, $W_{Q},W_{K}, W_{V}$ are learnable matrices.
The textual prompt is embedded with a T5 encoder and integrated using a cross-attention mechanism.
