# Supplementary material for: InstaDrive: Instance-Aware Driving World Models for Realistic and Consistent Video Generation
Source: arXiv:2602.03242 source file (2026-02-03)
Supplement: Supplementary file 5 [file Appendix-experiment.tex]

\section{More Experimental Details}  
\label{app: exp}

We provide a project page for additional video results: \url{https://metadrivescape.github.io/papers_project/InstaDrive/page.html}.

%\textcolor{red}{Please unzip the entire supplementary materials archive before opening the webpage. Tested OK on macOS and Windows 10 systems.}

\subsection{Training Details}
Our method is implemented based on OpenSora \cite{opensora}. 
Initially, we train for 20k iterations on the front-view videos from the NuScenes training set. Next, to adapt to multi-view positional encoding, we froze the backbone and fine-tuned the patch embedder for 2k iterations. Finally, we added all the control modules and trained the entire model for 100k iterations with a mini-batch size of 1. All training inputs were set to 16x256x448 and performed on 8 A100 GPUs. Additionally, during training, we set a 0.2 probability of not adding noise to the first frame and assigned a timestep of 0 to the first frame, enabling the model to have image-to-video generation capability. As a result, during testing, the model can autoregressively iterate. Experimental results show that our method can stably generate over 200 frames.% and the project webpage included.

\subsection{Perception Evaluation Details}
In Tab.~\ref{tab:perception_augment}, StreamPETR was re-implemented from official config due to resolution differences with Panacea. Stronger baselines are harder to surpass, further highlighting our data’s effectiveness.

%\subsection{Framework Details}

% We did not use OpenSora V1.2, even though this version offers better performance. This is because the VAE in V1.2 also compresses the temporal dimension, and we found that this temporal compression leads to significant detail loss when generating driving scenes. The likely reason is that driving scenarios typically involve fast motion, and compressing the temporal dimension results in the loss of too much information. How to achieve reasonable spatiotemporal compression for generating autonomous driving scenes might also be a topic worth further research.
