# Supplementary material for: InstaDrive: Instance-Aware Driving World Models for Realistic and Consistent Video Generation
Source: arXiv:2602.03242 source file (2026-02-03)
Supplement: Supplementary file 6 [file Appendix-limitations.tex]

\section{Limitations}

Our work establishes a robust, physically informed framework for generating high-quality, multi-view driving videos, achieving state-of-the-art performance in both video generation quality and downstream perception task validation. However, certain limitations remain, mainly due to time and resource constraints.  

Currently, our model's design has not been exhaustively optimized, leaving room for improvement in the quality of the generated videos. For example, the training process is conducted at a relatively low spatial resolution of $256 \times 448$, which constrains visual fidelity. Scaling to higher resolutions would require fine-tuning the position embeddings to ensure compatibility, an aspect not yet addressed in this work.  

Future research could explore the integration of more advanced generative models, such as SD-XL ~\cite{DBLP:journals/corr/abs-2307-01952}, and develop more efficient methods to produce high-fidelity videos at larger spatial resolutions. Additionally, the computational cost of inference for InstaDrive is relatively high, which presents another avenue for improvement. Enhancing the efficiency of InstaDrive will be a key focus in future developments to make the model more practical for real-world applications.
